# Supplementary material for: Discovering Biases in Information Retrieval Models Using Relevance Thesaurus as Global Explanation
Source: arXiv:2410.03584 source file (2024-10-04)
Supplement: Supplementary file 2 [file influential_terms.tex]

\newpage
\section{Relevance Thesaurus Entries}
\begin{equation}
     \text{idf}(qt) \cdot \text{tf}(qt) \cdot \text{tf}(dt) \cdot \text{score} \nonumber
\end{equation}
where $\text{idf}$ is inverse document frequency, and $\text{tf}$ is the term frequency in the collection.
\begin{center}
\tablehead{\toprule Query Term   & Doc Term     & Score \\ \hline}
\begin{supertabular}{c|c|c}
how          & average      & 0.52  \\
long         & years        & 0.70  \\
how          & per          & 0.52  \\
how          & usually      & 0.57  \\
how          & hour         & 0.59  \\
how          & days         & 0.60  \\
long         & hour         & 0.70  \\
how          & depend       & 0.52  \\
long         & month        & 0.69  \\
long         & days         & 0.85  \\
long         & week         & 0.73  \\
how          & minutes      & 0.70  \\
how          & typically    & 0.57  \\
old          & age          & 0.54  \\
how          & costs        & 0.56  \\
long         & minutes      & 0.77  \\
cost         & price        & 0.72  \\
when         & april        & 0.64  \\
when         & july         & 0.51  \\
when         & january      & 0.60  \\
when         & march        & 0.65  \\
how          & approximate  & 0.67  \\
when         & june         & 0.57  \\
call         & phone        & 0.62  \\
how          & length       & 0.58  \\
when         & august       & 0.58  \\
when         & september    & 0.55  \\
numbers      & number       & 0.60  \\
meaning      & definition   & 0.50  \\
costs        & cost         & 0.71  \\
much         & costs        & 0.59  \\
when         & february     & 0.65  \\
when         & november     & 0.52  \\
year         & april        & 0.59  \\
long         & length       & 0.69  \\
year         & january      & 0.56  \\
cost         & costs        & 0.89  \\
year         & march        & 0.61  \\
salary       & pay          & 0.51  \\
phone        & cell         & 0.57  \\
costs        & price        & 0.67  \\
length       & days         & 0.61  \\
pay          & costs        & 0.51  \\
number       & numbers      & 0.64  \\
price        & costs        & 0.68  \\
pay          & salary       & 0.59  \\
how          & median       & 0.61  \\
cell         & phone        & 0.60  \\
cost         & fee          & 0.57  \\
treat        & treatment    & 0.52  \\
paid         & pay          & 0.53  \\
weather      & temperature  & 0.87  \\
year         & february     & 0.58  \\
length       & minutes      & 0.67  \\
food         & meat         & 0.59  \\
average      & median       & 0.55  \\
phone        & contact      & 0.61  \\
contact      & phone        & 0.69  \\
long         & minute       & 0.62  \\
how          & seconds      & 0.56  \\
fee          & costs        & 0.53  \\
definition   & noun         & 0.69  \\
definition   & dictionary   & 0.56  \\
means        & noun         & 0.55  \\
points       & point        & 0.51  \\
refer        & noun         & 0.50  \\
climate      & temperature  & 0.77  \\
long         & seconds      & 0.66  \\
weather      & cold         & 0.60  \\
meaning      & noun         & 0.61  \\
minute       & minutes      & 0.51  \\
how          & cent         & 0.52  \\
point        & points       & 0.52  \\
die          & death        & 0.56  \\
food         & restaurant   & 0.57  \\
food         & grain        & 0.52  \\
word         & noun         & 0.57  \\
fast         & speed        & 0.62  \\
open         & opening      & 0.54  \\
waters       & water        & 0.50  \\
animal       & dog          & 0.58  \\
call         & calling      & 0.67  \\
define       & noun         & 0.61  \\
long         & duration     & 0.60  \\
minutes      & minute       & 0.53  \\
weigh        & weight       & 0.56  \\
how          & min          & 0.51  \\
woman        & women        & 0.55  \\
mean         & noun         & 0.55  \\
call         & telephone    & 0.62  \\
run          & running      & 0.63  \\
bases        & base         & 0.52  \\
climate      & weather      & 0.71  \\
mobile       & phone        & 0.58  \\
words        & noun         & 0.57  \\
pay          & wage         & 0.66  \\
technique    & method       & 0.57  \\
weather      & winter       & 0.70  \\
periods      & period       & 0.57  \\
animal       & dogs         & 0.68  \\
food         & dish         & 0.60  \\
\end{supertabular}
\end{center}
